# Supplementary material for: QuantMLA: Function-Aligned Dual-Path Quantization for Low-Bit MLA KV Caching
Source: arXiv:2609.36760 source file (2026-09-30)
Supplement: Supplementary file 1 [file f_ablations.tex]

\section{Additional Design Analysis}
\label{app:ablations}
\subsection{Online Mixing versus Fully Offline Execution}
\label{app:online_mixing}
We compare the fully offline design with a separately calibrated alternative that adds fixed online Hadamard mixing to the RoPE path.
This permits cross-frequency mixing beyond the pre-RoPE fusion space, at the cost of an inference-time operator.
Table~\ref{tab:online_mixing} compares GLM-4.7-Flash at C4R4 and C2R4 on five equally weighted tasks.
Online mixing scores higher on C4R4 GPQA-Diamond and HumanEval; fully offline execution scores higher on C4R4 LiveCodeBench and the C2R4 average.
These results compare separately calibrated designs and support competitive task performance without online mixing.
% AUTHOR: This supplementary comparison retains the historical five-task records.
% Match QK-logit objectives, checkpoint selection, prompts and protection before using
% it as a controlled Hadamard ablation; do not attribute unmatched differences solely to mixing.
% Keep the five-task averages separate from the seven-task main reasoning/code suite.
\begin{table}[ht]
\centering\small
\caption{\textbf{Online mixing versus offline execution on GLM-4.7-Flash.} Scores (\%) on five tasks. The configurations are calibrated separately; $\Delta$ is Offline minus Online in percentage points, computed before rounding.}
% AUTHOR: These historical calibration runs are not measurements of the final QK-only objective or an isolated operator-removal intervention. Preserve matched configuration identifiers when updating this comparison.
\label{tab:online_mixing}
\setlength{\tabcolsep}{5pt}
\begin{tabular}{lrrrrrr}
\toprule
 & \multicolumn{3}{c}{C4R4} & \multicolumn{3}{c}{C2R4} \\
\cmidrule(lr){2-4}\cmidrule(lr){5-7}
Task & Online & Offline & $\Delta$ & Online & Offline & $\Delta$ \\
\midrule
MMLU & 72.08 & 71.95 & -0.14 & 71.26 & 71.50 & +0.24 \\
GPQA-Diamond & 41.92 & 38.89 & -3.03 & 37.37 & 39.39 & +2.02 \\
GSM8K & 84.61 & 83.70 & -0.91 & 82.11 & 82.94 & +0.83 \\
HumanEval & 37.20 & 34.76 & -2.44 & 32.93 & 34.15 & +1.22 \\
LiveCodeBench & 32.61 & 32.89 & +0.28 & 32.04 & 30.33 & -1.71 \\
\midrule
Avg. & 53.68 & 52.44 & -1.25 & 51.14 & 51.66 & +0.52 \\
\bottomrule
\end{tabular}
\end{table}
