# Supplementary material for: QuantMLA: Function-Aligned Dual-Path Quantization for Low-Bit MLA KV Caching
Source: arXiv:2609.36760 source file (2026-09-30)
Supplement: Supplementary file 2 [file h_limitations.tex]

\section{Limitations}
\label{app:limitations}
Our model analyzes perturbations at a fixed attention layer and in declared cache coordinates; it does not determine end-to-end accuracy rankings.
Positional QK reconstruction controls an output-error bound without equaling output reconstruction, and separately learned paths can interact after composition.
Cross-method results compare complete configurations, including BF16 protection, rather than transformations alone.
Benchmark averages do not establish preservation of every task, long-form behavior, safety property, or agent capability, nor transfer to other attention architectures.
Finally, serving gains depend on the model, memory budget, batch size, and workload; operator speedups need not transfer proportionally to throughput.
